# Supplementary material for: ChartMimic: Evaluating LMM's Cross-Modal Reasoning Capability via Chart-to-Code Generation
Source: arXiv:2406.09961 source file (2025-02-28)
Supplement: Supplementary file 1 [file appx.trycatch.tex]

\section{TryCatch}
Additionally, our preliminary experiments revealed that the code generated by many open-source LMMs often fails to execute correctly, rendering them unable to produce images, resulting in mostly zero scores.
Therefore, we handle code execution errors by adding ``\texttt{matplotlib.savefig(format=`pdf')}'' in the ``\texttt{except}'' block of a ``\texttt{try-except}'' statement to force rendering and obtain the correct execution results before the error occurred.
\newpage
